# Supplementary material for: Every Parameter Matters: Ensuring the Convergence of Federated Learning with Dynamic Heterogeneous Models Reduction
Source: arXiv:2310.08670 source file (2023-10-26)
Supplement: Supplementary file 1 [file 4Results_CIFAR.tex]

\section{More Results For CIFAR-10-IID}

In this section we present more supplementary experimental results on CIFAR 10 dataset to test the effects of pruning on convolutional layers. Specifically, we present the training progress in respect of global loss and accuracy for selected pruning techniques where we focus on WP and FS. 

\subsection{Change of Notations}
In the main paper we use code name for simplicity of notation and better understanding. Here we present the results with their detailed settings.

For a full model without pruning it can be described as 
$\mathbb{P}_{1} (\theta)=  \{\textsl{S}_{1},\textsl{S}_{2},\textsl{S}_{3},\textsl{S}_{4}\}$, where
$$m_{i} = 1 \ \text{if} \ \theta_{i}\in \{\textsl{S}_{1}\cup \textsl{S}_{2}\cup \textsl{S}_{3}\cup \textsl{S}_{4}\} \ \text{ otherwise} \ m_{i} = 0$$.
As we have demonstrated the effects of pruning MLP layers, on CIFAR10 datasets we focus on the effects of conv2d layers.

We have another 3 pruning polices for conv2d layers as follows:
$$\mathbb{P}_{2} (\theta)=  \{\textsl{S}_{1},\textsl{S}_{3},\textsl{S}_{4}\}$$
$$\mathbb{P}_{3} (\theta)=  \{\textsl{S}_{1},\textsl{S}_{2},\textsl{S}_{4}\}$$
$$\mathbb{P}_{4} (\theta)=  \{\textsl{S}_{1},\textsl{S}_{2},\textsl{S}_{3}\}$$

For WP and PT, when using $\mathbb{P}_{2}$ the top 75\% of kernels will be kept,  i.e. for the first conv2d layer, the 5 largest kernels out of total of 6 kernels will be kept, and the 6-th kernel will be pruned. Under all pruning polices MLP layers will be pruned at 75\% accordingly. Note under such settings, code name without full model '1' , e.g. '2222333444', will not satisfy our necessary condition of convergence.

For FS, we denote $\mathbb{P}_{2}$ as the similar policy as above but only the first continuous parameters, i.e. for the first conv2d layer, the first 5 kernels out of total of 6 kernels will be kept, and the 6-th kernel will be pruned, together with pruning MLP layers at 75\%. We denote $\mathbb{P}_{3}$ as only pruning conv2d layers and $\mathbb{P}_{4}$ as only pruning MLP layers. In this case, note that even with same codename for WP and FS, their results are NOT directly comparable.

And we further denote a local client with its pruning policy, as an example, the case "*WP-M1" uses 4 local clients with full models, 2 local clients with pruned models using pruning policy  $\mathbb{P}_{4}$, 2 local clients with pruned models using pruning policy $\mathbb{P}_{2}$ and  2 local clients with pruned models using pruning policy $\mathbb{P}_{3}$, then we denote its code name as "1111223344" for simpler notation. Note that we continue to use code name "FedAvg" as a baseline rather than "1111111111". For the rest of the appendix we continue using such notations for denoting its pruning policy settings. For the final training results we focus on WP, FS and NP as PT is not found competitive without a carefully designed algorithm, however we still keep the training details for PT.

\begin{table}[]
\centering
\resizebox{\textwidth}{!}{%
\begin{tabular}{@{}llcccc@{}}
\toprule
Codename   & PARAs(K)        & \%   & FLOPs(K) & \%   & Testing Accuracy \\ \midrule
1111111111 & 512.80           & 1.00 & 653.8    & 1.00 & 53.63            \\
1111111122 & 482.34          & 0.94 & 619.6    & 0.94 & 53.12            \\
1111112222 & 451.936         & 0.88 & 587.0    & 0.89 & 52.66            \\
1111112223 & 451.936         & 0.88 & 587.0    & 0.89 & 52.98            \\
1111112233 & 451.936         & 0.88 & 587.0    & 0.89 & 54.20            \\
1111113333 & 451.936         & 0.88 & 587.0    & 0.89 & 52.96            \\
1111114444 & 451.936         & 0.88 & 587.0    & 0.89 & 51.61            \\
1111222222 & 421.504         & 0.82 & 553.7    & 0.84 & 51.69            \\
1111222334 & 421.504         & 0.82 & 553.7    & 0.84 & 52.20            \\
1111223344 & 421.504         & 0.82 & 553.7    & 0.84 & 52.54            \\
1222333444 & 375.856         & 0.73 & 503.6    & 0.77 & 49.15            \\ \bottomrule
\end{tabular}%
}
\caption{Results For Weights Pruning on CIFAR 10}
\label{tab:my-table}
\end{table}

\begin{table}[]
\centering
\resizebox{\textwidth}{!}{%
\begin{tabular}{@{}llcccc@{}}
\toprule
Codename   & PARAs(K) & \%   & FLOPs(K) & \%   & Testing Accuracy \\ \midrule
1111111111 & 512.81   & 1.00 & 653.80   & 1.00 & 54.78            \\
1111111122 & 476.37   & 0.92 & 619.68   & 0.94 & 54.10             \\
1111112222 & 439.93   & 0.85 & 585.57   & 0.89 & 52.87            \\
1111113333 & 471.28   & 0.91 & 589.48   & 0.90 & 53.96            \\
1111113344 & 467.92   & 0.91 & 589.06   & 0.90 & 53.90             \\
1111114444 & 464.57   & 0.90 & 588.64   & 0.90 & 54.44            \\
1111222222 & 403.49   & 0.78 & 551.46   & 0.84 & 52.74            \\
2222333444 & 372.59   & 0.72 & 488.47   & 0.74 & 52.35            \\ \bottomrule
\end{tabular}%
}
\caption{Results For Fixed Sub-network on CIFAR 10}
\label{tab:my-table}
\end{table}

\begin{figure}[h]
     \centering
     \begin{subfigure}[b]{0.49\textwidth}
         \centering
         \includegraphics[width=\textwidth]{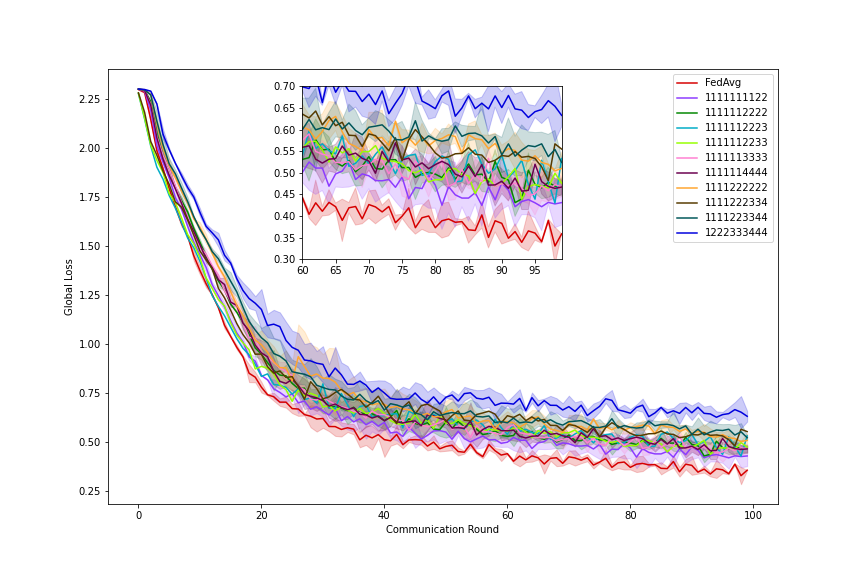}
         \caption{Global Loss}
         \label{fig:1}
     \end{subfigure}
     \hfill
     \begin{subfigure}[b]{0.49\textwidth}
         \centering
         \includegraphics[width=\textwidth]{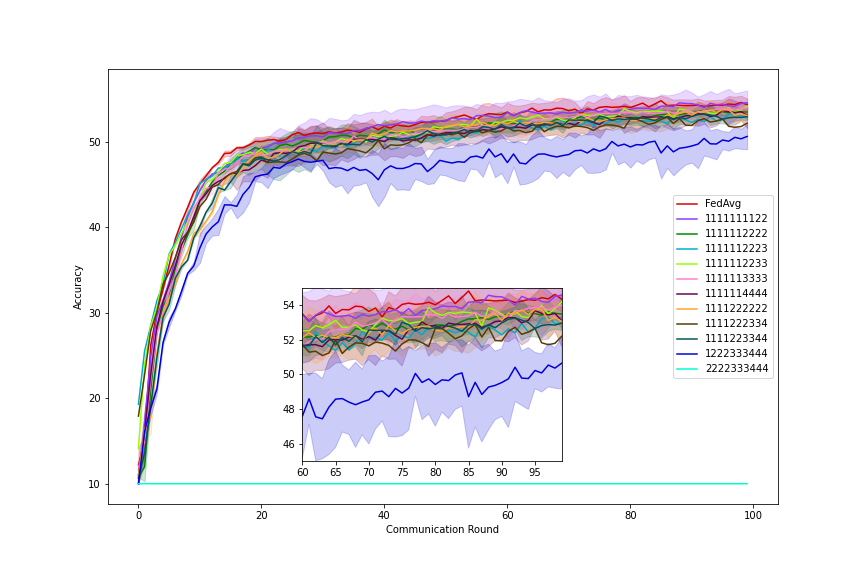}
         \caption{Accuracy}
         \label{fig:three sin x}
     \end{subfigure}
        \caption{Results on Weights Pruning on CIFAR10 IID}
        \label{fig:1}
\end{figure}

\begin{figure}[h]
     \centering
     \begin{subfigure}[b]{0.49\textwidth}
         \centering
         \includegraphics[width=\textwidth]{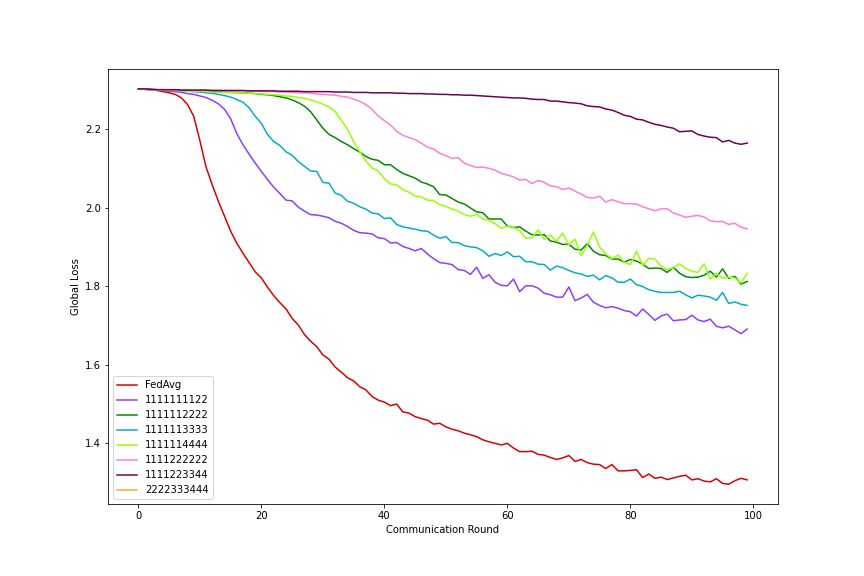}
         \caption{Global Loss}
         \label{fig:1}
     \end{subfigure}
     \hfill
     \begin{subfigure}[b]{0.49\textwidth}
         \centering
         \includegraphics[width=\textwidth]{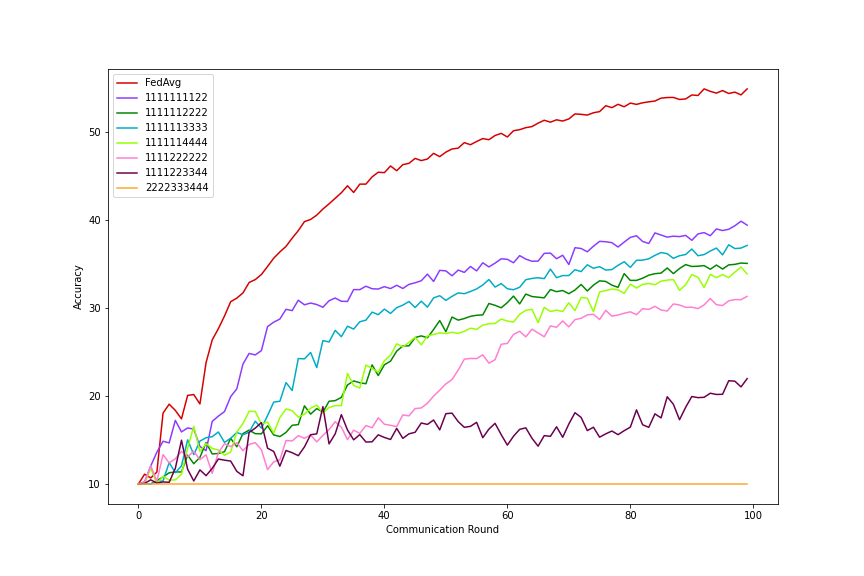}
         \caption{Accuracy}
         \label{fig:three sin x}
     \end{subfigure}
        \caption{Results on Pruning with pre-trained mask on CIFAR10 IID}
        \label{fig:1}
\end{figure}

\begin{figure}[h]
     \centering
     \begin{subfigure}[b]{0.49\textwidth}
         \centering
         \includegraphics[width=\textwidth]{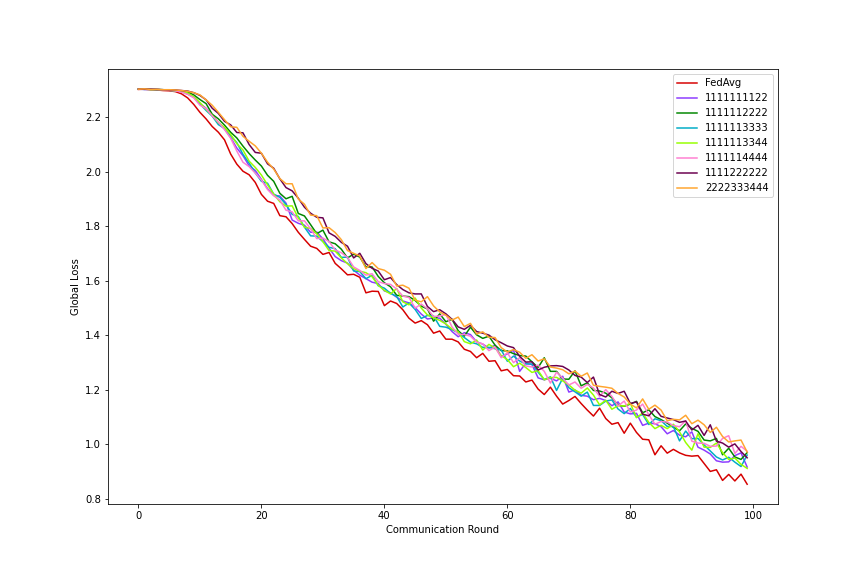}
         \caption{Global Loss}
         \label{fig:1}
     \end{subfigure}
     \hfill
     \begin{subfigure}[b]{0.49\textwidth}
         \centering
         \includegraphics[width=\textwidth]{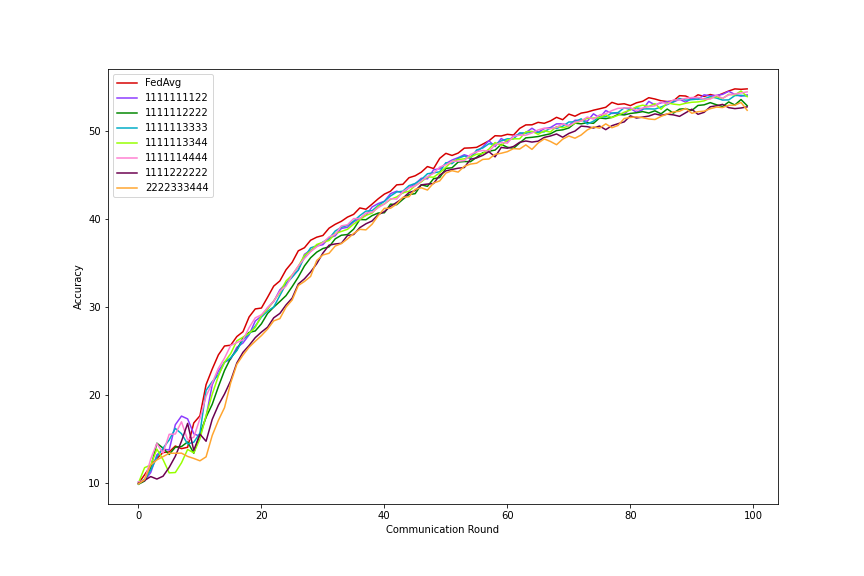}
         \caption{Accuracy}
         \label{fig:three sin x}
     \end{subfigure}
        \caption{Results on Fixed Sub-network Pruning on CIFAR10 IID}
        \label{fig:1}
\end{figure}
